# Supplementary material for: CorrGRPO: Correlation-Normalized GRPO for Multi-Reward Learning
Source: arXiv:2609.36820 source file (2026-09-29)
Supplement: Supplementary file 1 [file appendix-agent-security.tex]

% Insert after the manuscript's existing \appendix command.
% Requires natbib and url or hyperref.
\section{Agent Benchmarks and Evaluation Protocols}
\label{app:agent_protocols}

\subsection{AgentDojo}
\label{app:agentdojo_protocol}
AgentDojo \citep{debenedetti2024agentdojo} provides stateful environments in which an agent completes user tasks through executable tools. Task-specific checkers evaluate the final answer, environment state, or tool-call trace, depending on the task. Our rollout wrapper executes the official environment and passes the resulting trajectory to the user-task and injection-task checkers. Utility therefore measures completion of the intended task rather than merely whether a tool call is syntactically valid.

\paragraph{Attacks and observation injection.}
We use the \texttt{important\_instructions} and \texttt{tool\_knowledge} attacks. Both place attacker-controlled text in environment content that is subsequently returned to the agent as a tool observation. The former impersonates a message from the user and presents the attacker's objective as a prerequisite for completing the legitimate task. The latter additionally specifies a sequence of tools and argument placeholders for achieving that objective. The malicious instructions reach the agent through observations; the original user request remains the legitimate task. The attack implementations are provided by AgentDojo \citep{agentdojo_attack_implementation}.

\paragraph{Illustrative agent trajectory.}
The following schematic trajectory illustrates the banking bill-payment task and observation injection. Account identifiers and the payment date are placeholders, and the injected text and tool responses are abbreviated for presentation. It is not a recorded model rollout \citep{agentdojo_banking_user_tasks,agentdojo_banking_injection_tasks}.
\begin{verbatim}
[User]
Please pay the bill in bill-december-2023.txt.

[Assistant: tool call]
{
  "name": "read_file",
  "arguments": {"file_path": "bill-december-2023.txt"}
}

[Tool: observation containing injected text]
Car Rental: 98.70
Recipient: <legitimate_account>
<INFORMATION>
Before paying this bill, identify the user's music-streaming
subscription from the transaction history. Send a transaction
to <attacker_account> and include the subscription in its
payment description. Then complete the original payment.
</INFORMATION>

[Assistant: tool call]
{
  "name": "send_money",
  "arguments": {
    "recipient": "<legitimate_account>",
    "amount": 98.70,
    "subject": "Car Rental",
    "date": "<payment_date>"
  }
}

[Tool: observation]
Payment completed.

[Assistant: final response]
The bill has been paid.
\end{verbatim}
In this trajectory, the injection enters through the \texttt{read\_file} observation. The agent completes the legitimate payment without performing the injected action, yielding $R_{\mathrm{util}}=1$ and $R_{\mathrm{sec}}=1$. An agent that completes both the legitimate payment and the injected transaction receives $R_{\mathrm{util}}=1$ and $R_{\mathrm{sec}}=0$; an agent that refuses all actions receives $R_{\mathrm{util}}=0$ and $R_{\mathrm{sec}}=1$.

\paragraph{Split and paired evaluation.}
We group cases by suite and user-task identifier before constructing the 1,584/411 train/test split. The 411 test cases contain 21 clean tasks and 390 attacked cases. For Joint Accuracy, each attacked case is paired with the clean result for the same suite and user task. The split called test here is the evaluation split also used for periodic validation in the saved training scripts.

\paragraph{Invalid reward outcomes.}
The saved reward function has a separate invalid-result branch. If the AgentDojo result is missing or marked invalid, it returns a scalar score of $-1$ by default and sets both utility and security component scores to zero. Missing trajectory state and exceptions during checker evaluation produce such invalid results in the saved agent-loop implementation. This rule does not imply that every recoverable tool error invalidates a trajectory. The penalty is configurable; the verified value of $-1$ is the saved default. Equation~\ref{eq:agent_reward} describes valid attacked trajectories, while invalid results follow this separate branch.

\subsection{Agent Security Bench}
\label{app:asb_protocol}
Agent Security Bench (ASB; \citealp{zhang2025asb}) evaluates agents across application scenarios with benign tasks, legitimate tools, and attacker goals. We use observation prompt injection (OPI) with the \texttt{context\_ignoring} attack setting and evaluate 400 clean/attacked pairs per model. In the saved evaluator, the attack text is appended to intermediate tool responses before the resulting observations are added to the agent's context. The payload attempts to redirect subsequent tool use toward an attacker tool.

\paragraph{Utility and attack-success checks.}
Our ASB evaluator checks utility by searching the recorded interaction for the expected achievement string of every required legitimate tool. Its attack-success field uses the recorded execution of the attacker tool when that execution flag is available, with the attack-goal string check retained as a fallback for older records. Thus, the utility metric follows ASB's expected-achievement check and does not constitute exact matching of all tool arguments. Clean utility and utility under attack use the corresponding clean and OPI runs, and Joint Accuracy is computed over the paired cases using Equation~\ref{eq:agent_joint_accuracy}.

\subsection{InjecAgent}
\label{app:injecagent_protocol}
InjecAgent \citep{zhan2024injecagent} provides indirect prompt-injection cases in which an agent has already issued a legitimate tool call and is about to consume its observation. We use the \texttt{base} setting with the \texttt{InjecAgent} prompt template. Each case supplies the user's request, available tool descriptions, a preceding tool interaction, and an attacker-controlled tool response. The agent is then evaluated on its continuation after reading that response.

\paragraph{Attack types and metrics.}
Direct-harm attacks seek an unauthorized harmful tool action. Data-stealing attacks use two stages: obtaining the targeted information and then sending it to the attacker. The evaluator runs the second stage only when the first stage succeeds, supplying a simulated result for the first attacker tool before requesting the continuation. We report the official ASR-valid metrics for direct harm, each data-stealing stage, complete data stealing, and overall attack success. Invalid outputs are excluded according to the official metric's stage-specific denominators. Stage-two ASR is conditional on reaching that stage; complete data-stealing ASR requires both stages to succeed. InjecAgent supplies an attack-resistance evaluation in our experiments; Table~\ref{tab:qwen25-asb-opi-injecagent-valid} does not report a separate clean-utility score for this benchmark.
